# Supplementary material for: Reversing Single Sessions
Source: arXiv:1510.07253 source file (2016-04-08)
Supplement: Supplementary file 1 [file appendixCalculus.tex]

% !TEX root = ../reversible_sessions_TR.tex
\section{Proofs Section~\ref{sec:properties}}
\label{app:properties}

\subsection{Correspondence with \pic}
\label{app:Correspondence}

\lemmaApp{\ref{lem:str_preserved}}{
Let $M$ and $N$ be two \respi\ processes. If $M \congr N$ then $\forget{M} \congr \forget{N}$.
}
\begin{IEEEproof}
We proceed by induction on the derivation of $M \congr N$. For most of the laws 
in Figure~\ref{fig:congruence_respi} the conclusion is trivial because 
$\forget{M} \congr \forget{N}$ directly corresponds to a law for \pic\ in Figure~\ref{fig:congruence_pic}.
Instead, for the eighth and twelve laws, we easily conclude because by applying $\forgetMap$
we obtain the identity. 
\end{IEEEproof}

\bigskip

\lemmaApp{\ref{lem:correspondence}}{
Let $M$ and $N$ be two \respi\ processes. If $M \fwred N$ then $\forget{M} \red \forget{N}$.
}
\begin{IEEEproof}
We proceed by induction on the derivation of $M \fwred N$. Base cases:
\begin{itemize}
\item \rulelabel{fwCon}: We have that 
$M \ = \ \ptag{t_1}\requestAct{a}{x}{P_1}\ \mid \ \ptag{t_2}\acceptAct{a}{y}{P_2}$
\ \ and \ \ 
$N \ = \ \res{s,t_1',t_2'}(
	\ptag{t_1'}P_1\subst{\ce{s}}{x} \mid \ptag{t_2'}P_2\subst{s}{y}
	\mid \amem{\actEv{t_1}{\initAct{a}{x}{y}{P_1}{P_2}{s}}{t_2}}{t_1'}{t_2'})$
with $s,\ce{s} \notin \freese{P_1,P_2}$. By definition of $\forgetMap$, we obtain
$\forget{M} \ = \ \requestAct{a}{x}{P_1}\ \mid \ \acceptAct{a}{y}{P_2}$.
Now, by applying rules \rulelabel{Con} and \rulelabel{Str}, we have
$\forget{M} \red \res{s}(P_1\subst{\ce{s}}{x} \mid P_2\subst{s}{y} \mid \inact)\ =\ P$.
By definition of $\forgetMap$, we have $\forget{N}=P$ that permits to conclude.
\item \rulelabel{fwCom},\rulelabel{fwLab},\rulelabel{fwIf1},\rulelabel{fwIf2}: 
These cases are similar to the previous one.
\end{itemize}
Inductive cases:
\begin{itemize}
\item \rulelabel{fwPar}: We have that 
$M \ = \ M_1 \mid \ M_2$
\ \ and \ \
$N \ = \ M_1' \mid \ M_2$.
By the premise of rule \rulelabel{fwPar}, we also have $M_1 \ \fwred\ M_1'$ from which, 
by induction, we obtain
$\forget{M_1} \ \red\ \forget{M_1'}$.
By definition of $\forgetMap$, we get
$\forget{M}\ = \ \forget{M_1} \mid \ \forget{M_2}$.
By applying rule \rulelabel{Par}, we have
$\forget{M} \red \forget{M_1'} \mid \ \forget{M_2} \ =\ P$.
Thus, by definition of $\forgetMap$, we have
$\forget{N} \ = \ P$ that directly permits concluding.
\item \rulelabel{fwRes}: 
This case is similar to the previous one; in particular, when the restricted name is a tag, 
it is not even necessary to apply rule \rulelabel{Res}, because the forgetful map erases 
the restriction.
\item \rulelabel{fwStr}: 
By the premise of rule \rulelabel{fwStr}, we have 
$M  \congr M'$,
$M' \fwred N'$
and $N'  \congr N$.
By induction, we obtain
$\forget{M'} \red \forget{N'}$. 
By applying Lemma~\ref{lem:str_preserved},
we have $\forget{M}  \congr \forget{M'}$ and $\forget{N'} \congr \forget{N}$
that allow us to conclude.
\end{itemize}
\end{IEEEproof}

\bigskip

\lemmaApp{\ref{lem:str_preserved_inv}}{
Let $P$ and $Q$ be two \pic\ processes. If $P \congr Q$ then for 
any \respi\ process $M$ such that $\forget{M}=P$ there exists a \respi\ process
$N$ such that $\forget{N}=Q$ and $M \congr N$.
}
\begin{IEEEproof}
The proof is straightforward. Indeed, given a \respi\ process $M$ such that $\forget{M}=P$,
it must have the form $\res{\tuple{t}}(\ptag{t}P \mid \prod_{i\in I}m_i)$ up to $\congr$. Thus, 
the process $N$, such that $\forget{N}=Q$, can be defined accordingly: 
$N \congr \res{\tuple{t}}(\ptag{t}Q \mid \prod_{i\in I}m_i)$. Now, we can conclude 
by exploiting the ninth law in Figure~\ref{fig:congruence_respi}, 
i.e. $\ptag{t}P \congr \ptag{t}Q$\ \ if $P \congr Q$, and the fact that relation $\congr$ on
\respi\ processes is a congruence. 
\end{IEEEproof}

\bigskip

\lemmaApp{\ref{lem:correspondence_inv}}{
Let $P$ and $Q$ be two \pic\ processes. If $P \red Q$ then 
for any \respi\ process $M$ such that $\forget{M}=P$ there exists a \respi\ process
$N$ such that $\forget{N}=Q$ and $M \fwred N$.
}
\begin{IEEEproof}
We proceed by induction on the derivation of $P \red Q$. Base cases:
\begin{itemize}
\item \rulelabel{Con}: We have that 
$P \, = \, \requestAct{a}{x}{P_1} \mid \acceptAct{a}{y}{P_2}$
 \ and\ \
$Q \, = \, \res{s}(P_1\subst{\ce{s}}{x} \mid P_2\subst{s}{y})$ 
with $s,\ce{s} \notin \freese{P_1,P_2}$.
Let $M$ be a \respi\ process such that $\forget{M}=P$, it must have the form 
$\res{\tuple{t}}(\ptag{t_1}\requestAct{a}{x}{P_1} \mid \ptag{t_2}\acceptAct{a}{y}{P_2} \mid \prod_{i\in I}m_i)$ up to $\congr$. Thus, by applying rules \rulelabel{fwCon}, \rulelabel{fwPar}, \rulelabel{fwRes} and \rulelabel{fwStr}, 
we get $M \fwred \res{\tuple{t},s,t_1',t_2'}(
\ptag{t_1'}P_1\subst{\ce{s}}{x} \mid \ptag{t_2'}P_2\subst{s}{y}
\mid \amem{\actEv{t_1}{\initAct{a}{x}{y}{P_1}{P_2}{s}}{t_2}}{t_1'}{t_2'} \mid \prod_{i\in I}m_i) \, =\, N$.
We conclude by applying $\forgetMap$ to $N$, since we obtain $\forget{N}=Q$.
\item \rulelabel{Com},\rulelabel{Lab},\rulelabel{If1},\rulelabel{If2}: 
These cases are similar to the previous one.
\end{itemize}
Inductive cases:
\begin{itemize}
\item \rulelabel{Par}: We have that 
$P \ = \ P_1 \mid P_2$
\ \ and \ \
$Q \ = \ P_1' \mid P_2$.
Let $M$ be a \respi\ process such that $\forget{M}=P_1 \mid P_2$. 
We have $M \congr \res{\tuple{t}}(\ptag{t_1}P_1 \mid \ptag{t_2}P_2 \mid  \prod_{i\in I}m_i)
\congr \res{\tuple{t'}}(M_1 \mid \ptag{t_2}P_2 \mid  \prod_{j\in J}m_j)$
with $M_1\congr  \res{\tuple{t''}}(\ptag{t_1}P_1 \mid \prod_{k\in K}m_k)$,
$\tuple{t}=\tuple{t'},\tuple{t''}$ and $J\cup K=I$.
By the premise of rule \rulelabel{Par}, we also have $P_1 \red P_1'$ from which, 
by induction, since $\forget{M_1}=P_1$, 
there exists $M_1'$ such that $\forget{M_1'}=P_1'$ and $M_1 \fwred M_1'$.
Thus, by applying rules \rulelabel{fwPar}, \rulelabel{fwRes} and \rulelabel{fwStr}, 
we get 
$M \fwred  \res{\tuple{t'}}(M_1' \mid \ptag{t_2}P_2 \mid  \prod_{j\in J}m_j)\,=\,N$.
We conclude by applying $\forgetMap$ to $N$, because
$\forget{N}=\forget{M_1'} \mid P_2= P_1' \mid P_2 =Q$.
\item \rulelabel{Res}: 
This case is similar to the previous one.
\item \rulelabel{Str}: We have that 
$P \congr P'$, $Q \congr Q'$ and $P' \red Q'$.
Let $M$ be a process such that $\forget{M}=P$.
By applying Lemma~\ref{lem:str_preserved_inv}, 
there exists $M'$ such that $\forget{M'}=P'$ and $M \congr M'$.
By induction, there is $N'$ such that $\forget{N'}=Q'$ and $M' \fwred N'$.
By applying Lemma~\ref{lem:str_preserved_inv} again, 
there exists $N$ such that $\forget{N}=Q$ and $N \congr N'$.
By applying rule \rulelabel{fwStr}, we conclude $M \fwred N$.
\end{itemize}
\end{IEEEproof}

\subsection{Loop lemma}
\label{app:LoopLemma}

\lemmaApp{\ref{lemma:loop}}{
Let $M$ and $N$ be two reachable \respi\ processes. 
$M \fwred N$ if and only if $N \bwred M$.
}
\begin{IEEEproof}
The proof for the \emph{if} part is by induction on the derivation of $M \fwred N$.
Base cases:
\begin{itemize}
\item \rulelabel{fwCon}: We have that 
$M \ = \ \ptag{t_1}\requestAct{a}{x}{P_1}\ \mid \ \ptag{t_2}\acceptAct{a}{y}{P_2}$
\ \ and \ \ 
$N \ = \ \res{s,t_1',t_2'}(
	\ptag{t_1'}P_1\subst{\ce{s}}{x} \mid \ptag{t_2'}P_2\subst{s}{y}
	\mid \amem{\actEv{t_1}{\initAct{a}{x}{y}{P_1}{P_2}{s}}{t_2}}{t_1'}{t_2'})$
with $s,\ce{s} \notin \freese{P_1,P_2}$. 
By applying rule \rulelabel{bwCon}, we can directly conclude 
$N \bwred M$.
\item \rulelabel{fwCom},\rulelabel{fwLab},\rulelabel{fwIf1},\rulelabel{fwIf2}: 
These cases are similar to the previous one.
\end{itemize}
Inductive cases:
\begin{itemize}
\item \rulelabel{fwPar}: We have that 
$M  =  N_1 \mid N_2$, $N  = N_1' \mid N_2$ and $N_1 \fwred N_1'$.
By induction $N_1' \bwred N_1$. Thus, we conclude by applying rule \rulelabel{bwPar},
since we get $N  = N_1' \mid N_2 \bwred N_1 \mid N_2 = M$.
\item \rulelabel{fwRes} and \rulelabel{fwStr}: 
These cases can be proved by straightforwardly resorting to the induction hypothesis as in the previous case.
\end{itemize}

\noindent
The proof for the \emph{only if} part is by induction on the derivation of $N \bwred M$.
Base cases:
\begin{itemize}
\item \rulelabel{bwCon}: We have that 
$N \ = \ \res{s,t_1',t_2'}(\ptag{t_1'}P \mid \ptag{t_2'}Q 
	\mid$ 
	
	$
	 \amem{\actEv{t_1}{\initAct{a}{x}{y}{P_1}{P_2}{s}}{t_2}}{t_1'}{t_2'})$
\ \ and \ \ 
$M \ = \ \ptag{t_1}\requestAct{a}{x}{P_1}\ \mid \ \ptag{t_2}\acceptAct{a}{y}{P_2}$.
Since $N$ is a reachable process, memory $\amem{\actEv{t_1}{\initAct{a}{x}{y}{P_1}{P_2}{s}}{t_2}}{t_1'}{t_2'}$
has been generated by a synchronisation between threads
$\ptag{t_1}\requestAct{a}{x}{P_1}$ and $\ptag{t_2}\acceptAct{a}{y}{P_2}$,
producing a session channel $s$ and two continuation processes 
$P_1\subst{\ce{s}}{x}$ and $P_2\subst{s}{y}$ tagged by $t_1'$ and $t_2'$, respectively.
Now, by tag uniqueness implied by reachability and use of restriction in tag generation,
$P$ and $Q$ must coincide with $P_1\subst{\ce{s}}{x}$ and $P_2\subst{s}{y}$, respectively.
Therefore, by applying rule \rulelabel{fwCon}, we can directly conclude $M \fwred N$.
\item \rulelabel{bwCom},\rulelabel{bwLab},\rulelabel{bwIf}: 
These cases are similar to the previous one.
\end{itemize}
Inductive cases:
\begin{itemize}
\item \rulelabel{bwPar}: We have that 
$N  =  N_1 \mid N_2$, $M  = N_1' \mid N_2$ and $N_1 \bwred N_1'$.
By induction $N_1' \fwred N_1$. Thus, we conclude by applying rule \rulelabel{fwPar},
since we get $M  = N_1' \mid N_2 \fwred N_1 \mid N_2 = N$.
\item \rulelabel{bwRes} and \rulelabel{bwStr}: 
These cases can be proved by straightforwardly resorting to the induction hypothesis as in the previous case.
\end{itemize}
\end{IEEEproof}
